# Supplementary material for: Pairing boost from enhanced spin-fermion coupling in the pseudogap regime
Source: arXiv:2410.01705 ancillary file (2025-07-01)
Supplement: Supplementary file 1 [file supplement.pdf]

# Supplemental Material:

## Pairing boost from enhanced spin-fermion coupling in the pseudogap regime

Yang Yu,<sup>1</sup> Sergei Isakov,<sup>1</sup> Emanuel Gull,<sup>1</sup> Karsten Held,<sup>2</sup> and Friedrich Krien<sup>2</sup>

<sup>1</sup>*Department of Physics, University of Michigan, Ann Arbor, Michigan 48109, USA*

<sup>2</sup>*Institute for Solid State Physics, TU Wien, 1040 Vienna, Austria*

In this supplementary material we define various quantities used in the main text and provide further supporting results. Specifically, in Sec. I we define the pairing susceptibility and show how it is computed within the dynamical cluster approximation (DCA) via the Bethe-Salpeter equation (BSE). In Sec. II we introduce a modified BSE, which allows us to investigate the impact of the spin-fermion vertex on pairing. Results for the eigenvalue spectra of both BSEs are provided in Sections I and II. In Sec. III we present additional results for the spin-fermion coupling, including the atomic limit, finite-size effects, weak coupling, a parametrization through an isotropic effective coupling constant, and modification of its static part. A brief comment on previous research regarding spin-fermion coupling is included at the end of Sec. III. In Sec. IV, we provide additional details, including the momentum tiling of the DCA clusters used in this study and supporting data related to the opening of the pseudogap.

### I. DIVERGENCE OF PAIRING SUSCEPTIBILITY AND EIGENVALUE ANALYSIS OF THE BETHE-SALPETER EQUATION

In this Section, we define the pairing susceptibility in Sec. IA and introduce its computational scheme in Sec. IB. We consider the eigenvalue spectrum of the BSE in Sec. IC.

#### A. Pairing susceptibility

In this work, we study the static homogeneous correlator  $P^d$  of the  $d_{x^2-y^2}$ -wave singlet pair field operator  $\hat{\Delta}^d$ . For a lattice system of  $N$  sites, it is defined as

$$P^d = \frac{1}{N} \int_0^\beta d\tau \left\langle \mathcal{T}_\tau \hat{\Delta}^d(\tau) \left[ \hat{\Delta}^d(0) \right]^\dagger \right\rangle, \quad (\text{S1})$$

where  $\beta = 1/T$  is the inverse temperature and  $\mathcal{T}_\tau$  represents the time-ordering operator for the imaginary time  $\tau$ .

The  $d_{x^2-y^2}$ -projected pair field operator is defined as  $\hat{\Delta}^d = \sum_{ij} \tilde{g}_{ij}^d (\hat{c}_{i\uparrow}\hat{c}_{j\downarrow} - \hat{c}_{i\downarrow}\hat{c}_{j\uparrow})$ , where  $\hat{c}_{i\uparrow(\downarrow)}$  annihilate an electron of spin  $\uparrow$  ( $\downarrow$ ) at lattice site  $i$ . We work on a two-dimensional lattice such that the location of site  $i$  is  $\mathbf{r}_i = (x_i, y_i)$ ; we use  $\hat{c}_{i\uparrow(\downarrow)}$  and  $\hat{c}_{\mathbf{r}_i\uparrow(\downarrow)}$  interchangeably below. The real space symmetry factor  $\tilde{g}_{ij}^d$  for the  $d_{x^2-y^2}$ -wave pairing on a square lattice reads [1]:

$$\tilde{g}_{ij}^d = \frac{1}{2} (\delta_{x_i, x_j \pm a} \delta_{y_i, y_j} - \delta_{x_i, x_j} \delta_{y_i, y_j \pm a}), \quad (\text{S2})$$

where  $a = 1$  is the lattice constant. Under the assumption of translation invariance of the lattice, the momentum space symmetry factor  $g_{\mathbf{k}}^d = \mathcal{F}_{\mathbf{k}}[\tilde{g}_{ij}^d]$  is obtained via Fourier transform as

$$\begin{aligned} g_{\mathbf{k}}^d &= \frac{1}{2} \sum_{(\mathbf{r}_i - \mathbf{r}_j)} e^{-i\mathbf{k}(\mathbf{r}_i - \mathbf{r}_j)} (\delta_{x_i, x_j+1} \delta_{y_i, y_j} + \delta_{x_i, x_j-1} \delta_{y_i, y_j} - \delta_{x_i, x_j} \delta_{y_i, y_j+1} - \delta_{x_i, x_j} \delta_{y_i, y_j-1}) \\ &= \frac{1}{2} (e^{ik_x} + e^{-ik_x} - e^{ik_y} - e^{-ik_y}) = \cos k_x - \cos k_y, \end{aligned} \quad (\text{S3})$$

where  $\mathbf{k} = (k_x, k_y)$ . Below we rewrite the definition of  $P^d$  in momentum-frequency notation and connect it to Ref. [2]. The fermionic momentum-frequency is defined as  $k = (\mathbf{k}, \nu)$  while the bosonic momentum-frequency index is defined as  $q = (\mathbf{q}, \omega)$ .

Under the assumption of space and time translational symmetry, we define the one-body Green's function in the momentum-frequency space as  $G_{k\sigma} = -\int_0^\beta \sum_{\mathbf{r}} d\tau e^{-i(k\mathbf{r} + \nu\tau)} \langle \mathcal{T}_\tau \hat{c}_{\mathbf{r}\tau\sigma} \hat{c}_{00\sigma}^\dagger \rangle$  where  $\sigma \in \{\uparrow, \downarrow\}$ . The  $\uparrow\downarrow$  and  $\uparrow\downarrow$  generalized

susceptibilities in the particle-particle channel are defined as

$$\chi_{kk'q,\uparrow\downarrow}^{\text{pp}} = \sum_{\mathbf{r}_1 \mathbf{r}_2 \mathbf{r}_3} \int_0^\beta d\tau_1 \int_0^\beta d\tau_2 \int_0^\beta d\tau_3 e^{-i\mathbf{k}\mathbf{r}_1 - i\nu\tau_1} e^{-i(\mathbf{q}-\mathbf{k})\mathbf{r}_2 - i(\omega-\nu)\tau_2} e^{i(\mathbf{q}-\mathbf{k}')\mathbf{r}_3 + i(\omega-\nu')\tau_3} \left\langle \mathcal{T}_\tau \hat{c}_{\mathbf{r}_1\tau_1\uparrow} \hat{c}_{\mathbf{r}_2\tau_2\downarrow} \hat{c}_{\mathbf{r}_3\tau_3\uparrow}^\dagger \hat{c}_{00\downarrow}^\dagger \right\rangle \quad (\text{S4a})$$

$$+ \beta N G_{k\uparrow} G_{k'\downarrow} \delta_{q-k-k',0},$$

$$\chi_{kk'q,\uparrow\downarrow}^{\text{pp}} = \sum_{\mathbf{r}_1 \mathbf{r}_2 \mathbf{r}_3} \int_0^\beta d\tau_1 \int_0^\beta d\tau_2 \int_0^\beta d\tau_3 e^{-i\mathbf{k}\mathbf{r}_1 - i\nu\tau_1} e^{-i(\mathbf{q}-\mathbf{k})\mathbf{r}_2 - i(\omega-\nu)\tau_2} e^{i(\mathbf{q}-\mathbf{k}')\mathbf{r}_3 + i(\omega-\nu')\tau_3} \left\langle \mathcal{T}_\tau \hat{c}_{\mathbf{r}_1\tau_1\uparrow} \hat{c}_{\mathbf{r}_2\tau_2\downarrow} \hat{c}_{\mathbf{r}_3\tau_3\downarrow}^\dagger \hat{c}_{00\uparrow}^\dagger \right\rangle. \quad (\text{S4b})$$

The generalized singlet susceptibility is defined according to Ref. [2] as

$$\chi_{kk'q}^{\text{si}} = \frac{1}{2} \left( \chi_{kk'q,\uparrow\downarrow}^{\text{pp}} - \chi_{kk'q,\uparrow\downarrow}^{\text{pp}} - \chi_{kk'q}^{\text{pp},0} \right), \quad (\text{S5})$$

where the bubble diagram reads

$$\chi_{kk'q}^{\text{pp},0} = \beta N G_{k\uparrow} G_{(q-k)\downarrow} \delta_{k,k'}. \quad (\text{S6})$$

We refer to the static homogeneous limit of  $\chi^{\text{si}}$  as,

$$P_{kk'} = \chi_{kk'0}^{\text{si}}. \quad (\text{S7})$$

Using SU(2) and translation symmetry one can show that

$$P^d = -\frac{4}{(\beta N)^2} \sum_{kk'} g_{\mathbf{k}}^d P_{kk'} (g_{\mathbf{k}'}^d)^*. \quad (\text{S8})$$

Using the crossing symmetry  $\chi_{k(q-k')q,\uparrow\downarrow}^{\text{pp}} = -\chi_{kk'q,\uparrow\downarrow}^{\text{pp}} + \chi_{kk'q}^{\text{pp},0}$ , one can also show that  $P^d = \frac{4}{(\beta N)^2} \sum_{kk'} g_{\mathbf{k}}^d \chi_{kk'0,\uparrow\downarrow}^{\text{pp}} (g_{\mathbf{k}'}^d)^*$ . This connects our formalism to the literature where  $\chi_{kk'0,\uparrow\downarrow}^{\text{pp}}$  was investigated, as, e.g., in Refs. [3–8].

## B. Dynamical cluster approximation

The dynamical cluster approximation (DCA) is an extension of dynamical mean field theory (DMFT) that captures short-to-intermediate range correlations. It maps a lattice model of size  $N$  onto a periodic cluster with  $N_c$  sites embedded in a self-consistent bath. The Brillouin zone of the lattice is divided into  $N_c$  patches, each centered around a cluster momentum, with  $\frac{N}{N_c}$  momentum points per patch. For more details on DCA see Refs. [4, 9, 10]. We use a continuous-time quantum Monte Carlo method as the impurity solver [11–14] which uses the submatrix updates technique [15]. In this text, we use lower-case symbols like  $\mathbf{k}$  for lattice momenta and upper-case symbols like  $\mathbf{K}$  for cluster momenta.

In DCA, we assume that the self-energy and the irreducible vertex function, obtained from the cluster solution, properly approximate the corresponding lattice quantities within the momentum patches around the corresponding cluster momenta. For instance, the lattice irreducible vertex function in the singlet channel,  $\Gamma_{kk'}$ , is approximated by the cluster irreducible vertex function,  $\Gamma_{KK'}^c$ , for all  $\mathbf{k} = \mathbf{K} + \tilde{\mathbf{k}}$  and  $\mathbf{k}' = \mathbf{K}' + \tilde{\mathbf{k}}'$  in the patches centered at  $\mathbf{K}$  and  $\mathbf{K}'$ . Here  $\tilde{\mathbf{k}}$  refers to the  $\frac{N}{N_c}$  wave vectors that connects  $\mathbf{K}$  and other points within the same patch.

The BSE for the lattice generalized pairing susceptibility reads [2]

$$P_{kk'} = -\chi_{kk'}^0 - \frac{1}{2(\beta N)^2} \sum_{k_1 k_2} \chi_{kk_1}^0 \Gamma_{k_1 k_2} P_{k_2 k'}. \quad (\text{S9})$$

In DCA, we define the coarse-grained generalized pairing susceptibility as  $\bar{P}_{KK'} = \frac{N_c^2}{N^2} \sum_{\tilde{\mathbf{k}} \tilde{\mathbf{k}}'} P_{(K+\tilde{\mathbf{k}})(K'+\tilde{\mathbf{k}}')}$ , where  $K + \tilde{\mathbf{k}} = (\mathbf{K} + \tilde{\mathbf{k}}, \nu)$ . Inserting the BSE for the lattice susceptibility, we get the BSE for the coarse-grained susceptibility

as

$$\begin{aligned}
\bar{P}_{KK'} &= \frac{N_c^2}{N^2} \sum_{\tilde{\mathbf{k}}\tilde{\mathbf{k}}'} P_{(K+\tilde{\mathbf{k}})(K'+\tilde{\mathbf{k}}')} \\
&= -\frac{N_c^2}{N^2} \sum_{\tilde{\mathbf{k}}\tilde{\mathbf{k}}'} \chi_{(K+\tilde{\mathbf{k}})(K'+\tilde{\mathbf{k}}')}^0 - \frac{1}{2(\beta N)^2} \frac{N_c^2}{N^2} \sum_{\tilde{\mathbf{k}}\tilde{\mathbf{k}}'} \sum_{k_1 k_2} \chi_{(K+\tilde{\mathbf{k}})k_1}^0 \Gamma_{k_1 k_2} P_{k_2(K'+\tilde{\mathbf{k}}')} \\
&\simeq -\frac{N_c^2}{N^2} \sum_{\tilde{\mathbf{k}}\tilde{\mathbf{k}}'} \chi_{(K+\tilde{\mathbf{k}})(K'+\tilde{\mathbf{k}}')}^0 - \frac{1}{2(\beta N)^2} \frac{N_c^2}{N^2} \sum_{\tilde{\mathbf{k}}\tilde{\mathbf{k}}'} \sum_{K_1 K_2} \sum_{\tilde{\mathbf{k}}_1 \tilde{\mathbf{k}}_2} \chi_{(K+\tilde{\mathbf{k}})(K_1+\tilde{\mathbf{k}}_1)}^0 \Gamma_{K_1 K_2}^c P_{(K_2+\tilde{\mathbf{k}}_2)(K'+\tilde{\mathbf{k}}')} \\
&= -\bar{\chi}_{KK'}^0 - \frac{1}{2(\beta N_c)^2} \sum_{K_1 K_2} \bar{\chi}_{KK_1}^0 \Gamma_{K_1 K_2}^c \bar{P}_{K_2 K'},
\end{aligned} \tag{S10}$$

where the coarse-grained bubble is defined as

$$\begin{aligned}
\bar{\chi}_{KK'}^0 &:= \frac{N_c^2}{N^2} \sum_{\tilde{\mathbf{k}}\tilde{\mathbf{k}}'} \chi_{(K+\tilde{\mathbf{k}})(K'+\tilde{\mathbf{k}}')}^0 \\
&= \frac{N_c^2}{N^2} \sum_{\tilde{\mathbf{k}}\tilde{\mathbf{k}}'} \beta N G_{(K+\tilde{\mathbf{k}})\uparrow} G_{(-K-\tilde{\mathbf{k}})\downarrow} \delta_{K+\tilde{\mathbf{k}}, K'+\tilde{\mathbf{k}}'} \\
&= \beta N_c \delta_{KK'} \frac{N_c}{N} \sum_{\tilde{\mathbf{k}}} G_{(K+\tilde{\mathbf{k}})\uparrow} G_{(-K-\tilde{\mathbf{k}})\downarrow}.
\end{aligned} \tag{S11}$$

In the main text and below, we focus on the coarse-grained quantities in DCA instead of lattice quantities. Therefore, to lighten the notation, we omit the overline on the coarse-grained quantities and the superscript ‘c’ for the cluster irreducible vertex:  $\bar{P}, \bar{\chi}^0, \Gamma^c \rightarrow P, \chi^0, \Gamma$ .

The BSE for the coarse-grained pairing susceptibility [Eq. (S11)] then reads in a  $K, K'$ -matrix notation

$$\hat{P} = -\hat{\chi}^0 - \frac{1}{2} \hat{\chi}^0 \hat{\Gamma} \hat{P}, \tag{S12}$$

where each matrix multiplication implies a prefactor of  $\frac{1}{\beta N_c}$ .

Finally, in the main text we split  $P^d$  into two parts: the bubble diagram part  $P_0^d$  and the vertex correction  $\mathcal{P}^d$ , which are defined as

$$P^d = P_0^d + \mathcal{P}^d = -\frac{4}{(\beta N_c)^2} \sum_{KK'} g_{\mathbf{K}}^d P_{KK'} (g_{\mathbf{K}'}^d)^*, \tag{S13a}$$

$$P_0^d = \frac{4}{(\beta N_c)^2} \sum_{KK'} g_{\mathbf{K}}^d \chi_{KK'}^0 (g_{\mathbf{K}'}^d)^*, \tag{S13b}$$

$$\mathcal{P}^d = -\frac{4}{(\beta N_c)^2} \sum_{KK'} g_{\mathbf{K}}^d (P_{KK'} + \chi_{KK'}^0) (g_{\mathbf{K}'}^d)^*. \tag{S13c}$$

### C. Eigenvalue analysis of the traditional Bethe-Salpeter equation

Equation (S12), or the analogous BSE for the  $\uparrow\downarrow$  channel, is frequently used to investigate pairing fluctuations. Hence, we refer to it as the *traditional* BSE. We can rewrite it as  $\hat{P} = -[\hat{1} + \frac{1}{2} \hat{\chi}^0 \hat{\Gamma}]^{-1} \hat{\chi}^0$ . By analyzing the eigenvalue equation,

$$-\frac{1}{2(\beta N_c)^2} \sum_{K_1 K_2} \chi_{KK_1}^0 \Gamma_{K_1 K_2} \phi_{K_2}^\alpha = \lambda^\alpha \phi_K^\alpha, \tag{S14}$$

often useful information about  $\hat{P}$  can be inferred from the leading eigenvalue  $\lambda^0$  and its corresponding eigenvector  $\phi^0$ . Previous studies of the  $\uparrow\downarrow$  channel, e.g. Refs. [3, 16, 17], have shown that the leading eigenvalue increases and approaches 1 as the temperature decreases, indicating a divergence in  $\hat{P}$ . It was found that  $\phi^0$  exhibits a  $d_{x^2-y^2}$ -wave

shape  $\propto \cos k_x - \cos k_y$  at low temperatures. Here, we provide further details on this eigenvalue analysis. While our focus is on the singlet channel, we confirm that our following conclusions remain the same when applied to the  $\uparrow\downarrow$  channel.

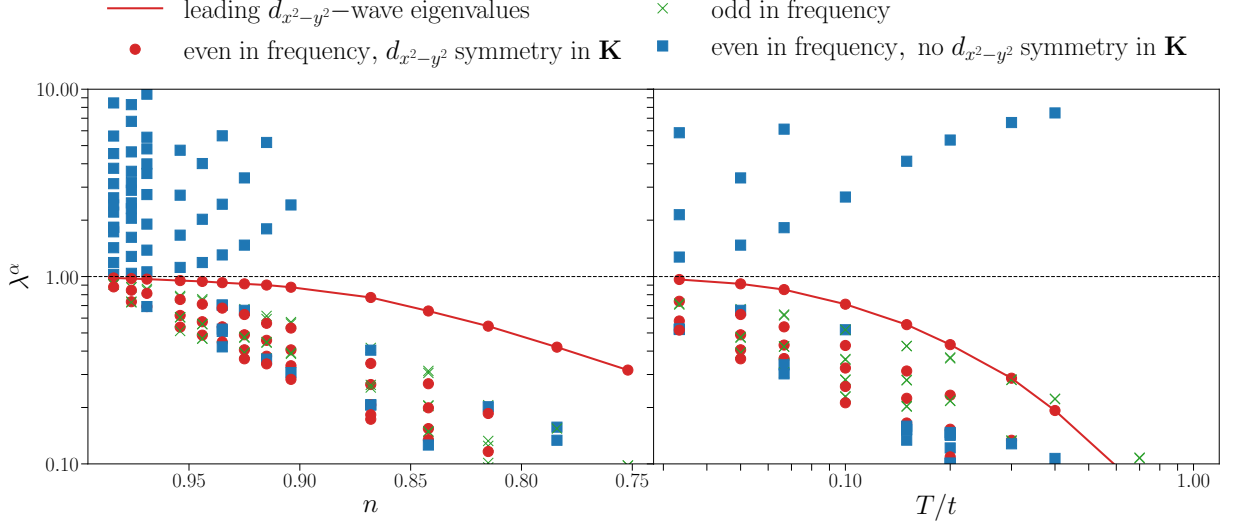

FIG. 1: Eigenvalue spectrum for the traditional BSE with parameters  $t = 1$ ,  $U = 7t$ , and  $t' = -0.15t$ . On the left, eigenvalues are shown for a density scan at  $T = 0.05t$ , and on the right, for a temperature scan at  $\delta = 0.075$ . For all densities  $n$  and temperatures  $T$  studied here, only eigenvalues between 0.1 and 10 are shown. The red line highlights the leading  $d_{x^2-y^2}$ -wave eigenvalues, while red circles mark all the  $d_{x^2-y^2}$ -wave eigenvalues. Blue squares indicate eigenvalues that are even in frequency but do not correspond to  $d_{x^2-y^2}$ -symmetry in momentum. Green crosses represent eigenvalues with eigenvectors odd in frequency, which do not contribute to pairing.

In Fig. 1 we present the eigenvalue spectra of the BSE as a function of doping (left,  $T = 0.05t$ ) or temperature (right,  $\delta = 0.075$ ), parameters are as in the main text. To satisfy the Pauli principle, all eigenvectors are either even or odd in frequency. Eigenvalues with odd-frequency eigenvectors (green crosses) do not contribute to  $d_{x^2-y^2}$ -wave pairing at all due to the summation over Matsubara frequencies  $\nu, \nu'$  in Eq. (S13). For eigenvalues with even-frequency eigenvectors, only those for which  $\sum_{\nu} \phi_{\mathbf{K}}$  has an overlap with  $g_{\mathbf{K}}^d$  contribute to  $P^d$  in Eq. (S13), see red circles in Fig. 1. Eigenvalues whose eigenvectors do not overlap with  $g_{\mathbf{K}}^d$  but are even in frequency are marked with blue squares.

We make two important observations in Fig. 1: (i) As shown in the left panel, for overdoping we observe results consistent with previous studies, where the leading eigenvalue has an even-frequency eigenvector and  $d_{x^2-y^2}$  symmetry in  $\mathbf{K}$  space. However, at lower doping levels, we see the emergence of some eigenvalues larger than 1, hence, the ‘leading’ eigenvalue is no longer of the  $d_{x^2-y^2}$  type. These large eigenvalues appear due to divergences of the irreducible vertex  $\Gamma$  in the charge and pairing channels [18–21]. A related discussion focusing on this type of eigenvalue spectra can be found in Section 3.1 of Ref. [17].

(ii) The leading eigenvalue with eigenvector of  $d_{x^2-y^2}$  symmetry does not exhibit a dome-like shape in the doping scan, at least for temperatures we explored. Instead, it remains close to 1 near half filling where the pairing susceptibility  $P^d$  is however diminished, see Fig. 2 in the main text. This may be the case due to the suppressed spectral weight in the pseudogap regime in combination with a strong pairing glue. Indeed, the bubble  $\hat{\chi}^0$  is small for underdoping, so that a sizable  $\hat{P}$  requires  $[\hat{1} + \frac{1}{2}\hat{\chi}^0\hat{\Gamma}]^{-1}$  to be very large. As the result, sizable pairing fluctuations in the pseudogap regime intrinsically require that the BSE converges only at a very high perturbation order; in other words, the corresponding eigenvalue must be very close to 1.

These observations undercut the usefulness of eigenvalue spectra in the considered regimes of the Hubbard model within DCA. Regarding (i), we notice that in either the doping or temperature scan, eigenvalues  $> 1$  appear in the spectrum for some value of  $n$  or  $T$ , respectively, without ever crossing 1 (presumably coming from  $+\infty$ ). Since a physical susceptibility diverges only for strictly  $\lambda = 1$ , we could, therefore, use this as a criterion for a phase transition. However, according to observation (ii) even an eigenvalue close to 1 does not necessarily signal the propensity to a phase transition. Therefore, our results in Fig. 1 imply that, except for the case of strictly  $\lambda = 1$ , which is challenging to achieve in numerical studies, we can not infer much from the eigenvalue spectrum of the traditional BSE at all. Neither the size of an eigenvalue, nor its trend as a function of doping or temperature is a reliable criterion for a phase transition [22].

## II. MODIFIED BETHE-SALPETER EQUATION

In this section, we derive a modified BSE that separates the ill-behaved part of the irreducible vertex  $\Gamma$  from spin fluctuations. As the result, large eigenvalues do not appear in the spectrum of the modified BSE. However, the  $d$ -wave eigenvalue still does not show the dome shape, for the same reasons discussed in the previous section regarding the eigenvalue spectra of the traditional BSE. This new formulation, nevertheless, provides a framework for testing the significance of the spin-fermion coupling. We emphasize that the modified BSE is fully equivalent to the standard BSE for calculating the pairing susceptibility, and every step of the derivation presented below is exact. The discussion of the corresponding eigenvalue spectra is purely illustrative. All results and conclusions presented in the main text are based on the physical pairing susceptibility and are independent of the eigenvalue spectra.

### A. Splitting spin-fluctuations from the Bethe-Salpeter equation

To derive the modified BSE, we employ the exact reformulation of the parquet formalism in terms of boson exchange introduced in Ref. [23]. The formulas for calculating the spin-fermion vertex  $\gamma_Q$  and the screened interaction in the spin channel,  $W_Q = -U + U^2 \chi_Q^{\text{sp}}$  [24], can be found in the supplemental material of Ref. [25].

Using Eqs. (12) and (18c) from Ref. [23] (we omit the superscripts ‘si’ and ‘sp’ used in the reference), we see that  $\Gamma$  can be expressed in terms of spin-fluctuation exchange and a rest,

$$\hat{\Gamma} = \hat{\Gamma}^{\text{sf}} + \hat{\Gamma}^{\text{r}}, \quad (\text{S15})$$

$$\Gamma_{KK'}^{\text{sf}} = -\frac{3}{2} \Delta_{KK', -K' - K} - \frac{3}{2} \Delta_{K, -K', K' - K} - 3U, \quad (\text{S16})$$

$$\Delta_{KK'Q} = \gamma_{KQ} W_Q \gamma_{K'Q}. \quad (\text{S17})$$

The screened interaction  $W$  and the spin-fermion vertex  $\gamma$  can be expressed through physical correlation functions [2], hence, they are free of divergences absent any phase transitions. The problematic part is therefore  $\Gamma^{\text{r}}$ . We get rid of it by summing a partial series before taking spin-fluctuation exchange into account.

First, we sum diagrams involving  $\Gamma^{\text{r}}$  only. To this end, we define

$$\hat{\chi}^{\text{r}} = -\hat{\chi}^0 - \frac{1}{2} \hat{\chi}^0 \hat{\Gamma}^{\text{r}} \hat{\chi}^{\text{r}}. \quad (\text{S18})$$

Solving for  $\chi^{\text{r}}$  by matrix inversion, the divergences of  $\Gamma^{\text{r}}$  simply turn into harmless zeros. Next, we invert Eqs. (S18) and (S12) and compare:

$$[\hat{\chi}^0]^{-1} = -[\hat{\chi}^{\text{r}}]^{-1} - \frac{1}{2} \hat{\Gamma}^{\text{r}}, \quad (\text{S19})$$

$$[\hat{\chi}^0]^{-1} = -\hat{P}^{-1} - \frac{1}{2} \hat{\Gamma}. \quad (\text{S20})$$

We subtract the first from the second line,

$$-\hat{P}^{-1} + [\hat{\chi}^{\text{r}}]^{-1} - \frac{1}{2} \hat{\Gamma}^{\text{sf}} = 0 \quad (\text{S21})$$

$$\Leftrightarrow \hat{P} = \hat{\chi}^{\text{r}} + \hat{\chi}^{\text{r}} \frac{1}{2} \hat{\Gamma}^{\text{sf}} \hat{P}. \quad (\text{S22})$$

Equation (S22) is the modified BSE. Solving for  $P$  leads to Eq. (3) in the main text.

### B. Absolute value of the spin-fermion vertex in the superconducting glue

We show that the spin-fluctuation glue for superconductivity depends only on the absolute value  $|\gamma|$  of the spin-fermion coupling. Due to inversion, time-reversal, and SU(2) symmetries, we have the relation  $\gamma_{KQ} = \gamma_{K+Q, -Q}$  [26]. In addition, complex conjugation yields  $\gamma_{KQ} = \gamma_{-K, -Q}^*$ . Therefore, we can express the two terms in Eq. (S16) as

$$\Delta_{KK', -K' - K}^{\text{sp}} = |\gamma_{K, -K' - K}|^2 W_{-K' - K}, \quad (\text{S23})$$

$$\Delta_{K, -K', K' - K}^{\text{sp}} = |\gamma_{K, K' - K}|^2 W_{K' - K}. \quad (\text{S24})$$

### C. Eigenvalue analysis of the modified Bethe-Salpeter equation

The modified BSE (S22) offers a clear way to study the impact of spin fluctuations and of the spin-fermion coupling on the pairing susceptibility, as illustrated in Fig. 2 of the main text. We supplement those results with an eigenvalue analysis of the modified BSE. The procedure is the same as in Sec. IC, except that the kernel  $-\frac{1}{2}\hat{\chi}^0\hat{\Gamma}$  is replaced with  $\frac{1}{2}\hat{\chi}^r\hat{\Gamma}^{\text{sf}}$ .

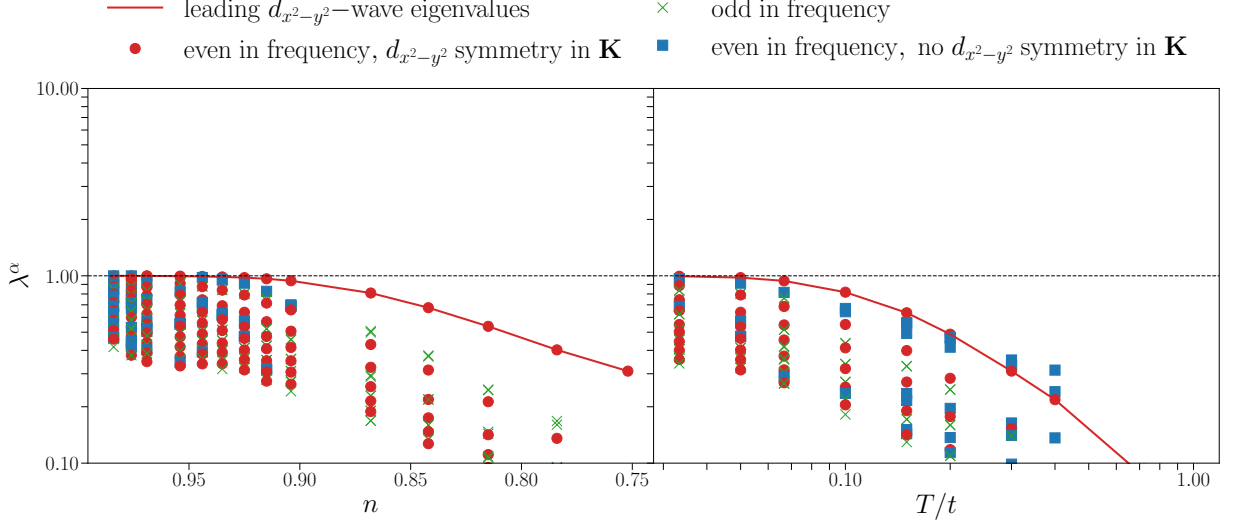

FIG. 2: Eigenvalue spectrum for the modified BSE with parameters  $t = 1$ ,  $U = 7t$ , and  $t' = -0.15t$ . In the left and right panels,  $T = 0.05t$  and  $\delta = 0.075$  are fixed, respectively. Symbols as in Fig. 1.

Figure 2 shows the eigenvalue spectrum of the modified BSE. Symbols identify properties of the corresponding eigenvectors as in Fig. 1. Unlike the traditional BSE, the modified BSE does not exhibit problematic large eigenvalues greater than 1 for any of the parameters explored, indeed, at low enough temperature the leading eigenvalue is of the  $d_{x^2-y^2}$ -wave type. However, the leading eigenvalue is still very close to 1 in the pseudogap regime, that is, even modest pairing fluctuations require a very high perturbation order of the modified BSE. Therefore, superconductivity in this regime should be studied looking at the pairing susceptibility  $P^d = P_0^d + \mathcal{P}^d$ , cf. Eq. (S13), where the modified BSE helps to evaluate the role of the spin-fermion coupling.

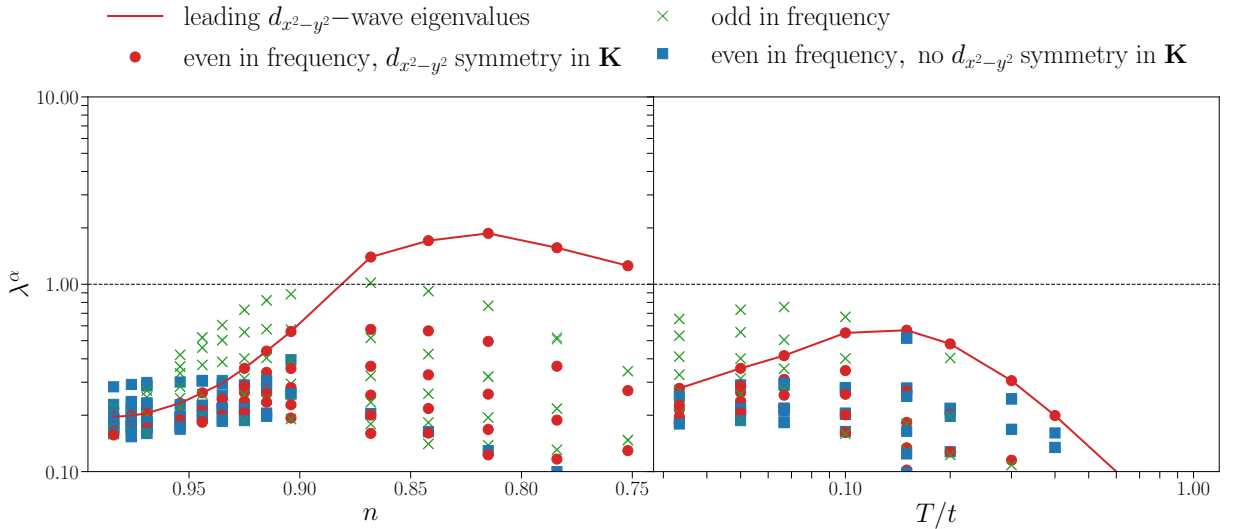

FIG. 3: Eigenvalue spectrum for the modified BSE with parameters  $t = 1$ ,  $U = 7t$ , and  $t' = -0.15t$  when  $|\gamma|$  is set to 1. In the left and right panels,  $T = 0.05t$  and  $\delta = 0.075$  are fixed, respectively. Symbols as in Fig. 1.

In the main text we considered setting  $|\gamma| = 1$ , Fig. 3 shows the eigenvalue spectrum of the modified BSE in this approximation. The red curve explains the behavior of the resulting  $\mathcal{P}_W^d$ , the green line in Fig. 2 of the main text. For  $|\gamma| = 1$ ,  $d_{x^2-y^2}$ -wave pairing is strongly suppressed in the pseudogap regime, but overestimated for overdoping ( $\lambda > 1$  in the left panel of Fig. 3 indeed implies that for overdoping a divergence of  $\mathcal{P}_W^d$  occurs for  $T > 0.05t$ .)

### III. ADDITIONAL RESULTS FOR THE SPIN-FERMION COUPLING

In this section we provide additional results for the spin-fermion coupling. In Sec. III A we consider this quantity in the atomic limit. We present results for 16-site DCA at strong coupling in Sec. III B and at weak coupling in Sec. III C. In Sec. III D we compare it to an analogous effective interaction  $\bar{U}/U$  considered in the literature.

#### A. Atomic limit

In the half-filled atomic limit,  $\hat{H} = U\hat{n}_\uparrow\hat{n}_\downarrow - \frac{U}{2}(\hat{n}_\uparrow + \hat{n}_\downarrow)$ , the magnetization  $\hat{n}_\uparrow - \hat{n}_\downarrow$  is a conserved quantity and we obtain  $\gamma$  through the Ward identity as described in Ref. [27].

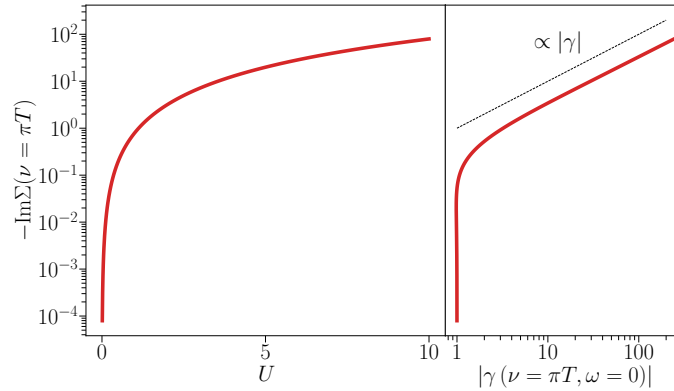

FIG. 4: Hubbard atom results at  $T = 0.1$ . Left: imaginary part of the antinodal self-energy at the first Matsubara frequency as a function of interacting  $U$ . Right: absolute value of the spin-fermion coupling plotted against the imaginary part of the self-energy.

The left and right panels of Fig. 4 show  $-\text{Im}\Sigma(\nu = \pi T) = \frac{U^2}{4\pi T}$  as a function of  $U$  and drawn against  $|\gamma(\nu = \pi T, \omega = 0)|$  for fixed  $T = 0.1$ . For  $-\text{Im}\Sigma(\nu = \pi T) \gg T$  this quantity is connected to  $|\gamma(\nu = \pi T, \omega = 0)|$  via a power law, albeit with the simple exponent 1. We note that in our DCA calculations for the Hubbard model (cf. Fig. 1 in the main text), we find approximately  $-\text{Im}\Sigma \propto |\gamma|^{0.7}$ .

#### B. Finite-size effects

To examine the effect of finite size, we present DCA calculation results on a larger cluster. Since the sign problem becomes more severe for larger clusters, we chose to perform the calculation at a higher temperature of  $T = 0.1t$ . A doping scan in the pseudogap regime is presented in Fig. 5.

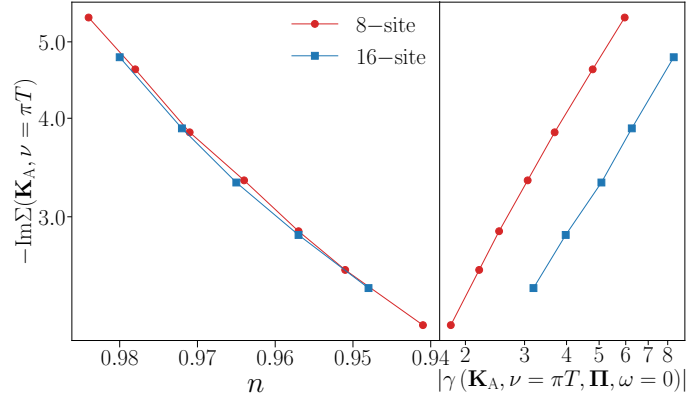

FIG. 5: Comparison of the 8-site and 16-site DCA calculation with parameters  $t = 1$ ,  $U = 7t$ ,  $t' = -0.15t$ , and  $T = 0.1t$ . Left: imaginary part of the antinodal self-energy at the first Matsubara frequency as a function of doping for 8-site (red circle) and 16-site (blue square) clusters. Right: absolute value of the spin-fermion coupling at the antinode plotted against the imaginary part of the self-energy.

As shown in the left panel, the imaginary part of the self-energy at the antinodal point  $\mathbf{K}_A$  for the first Matsubara frequency is very similar for the 8-site and 16-site clusters. However, in the right panel of Fig. 5, we see that the corresponding  $|\gamma|$  is larger for the 16-site cluster. This suggests that 8-site DCA may underestimate the enhancement of the coupling between antiferromagnetic spin fluctuations and antinodal fermions in the pseudogap regime.

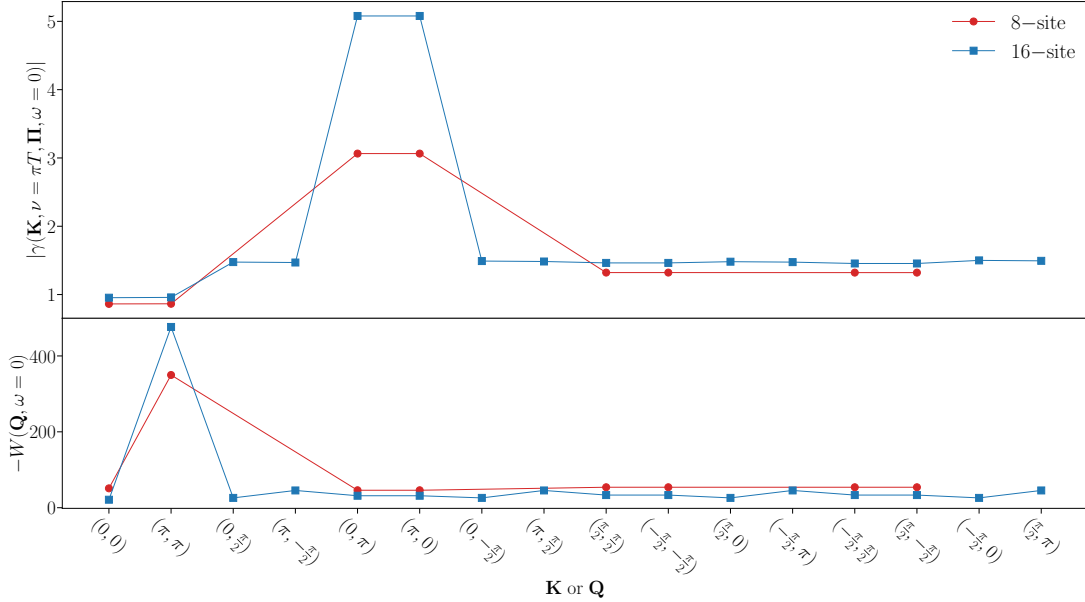

FIG. 6: Comparison of the 8-site and 16-site DCA calculation with parameters  $t = 1$ ,  $U = 7t$ ,  $t' = -0.15t$ ,  $T = 0.1t$  and  $n = 0.965$ . Top: absolute value of the spin-fermion coupling as a function of fermionic momentum  $\mathbf{K}$  for 8-site (red circle) and 16-site (blue square) clusters, with  $\mathbf{Q} = \mathbf{\Pi}$ . Bottom: magnitude of screened interaction as a function of bosonic momentum  $\mathbf{Q}$ .

In Fig. 6, we show the momentum dependence of the screened interaction  $W$  and of the spin-fermion coupling  $\gamma$  for  $n \approx 0.965$ . These quantities define the spin-fluctuation glue  $\Gamma^{\text{sf}}$  [cf. Eqs. (S16) and (S17)]. The bottom panel shows that for both the 8-site and 16-site clusters,  $W$  peaks at the antiferromagnetic wave vector  $\mathbf{Q} = \mathbf{\Pi} = (\pi, \pi)$ . In the top panel, with  $\mathbf{Q} = \mathbf{\Pi} = (\pi, \pi)$  fixed, we show how  $|\gamma|$  varies with the momentum  $\mathbf{K}$ . At the antinode,  $\mathbf{K} = (\pi, 0)$  or  $(0, \pi)$ , which corresponds to the locus of the peak, the 16-site cluster exhibits a larger value compared to the 8-site cluster.

### C. Weak coupling

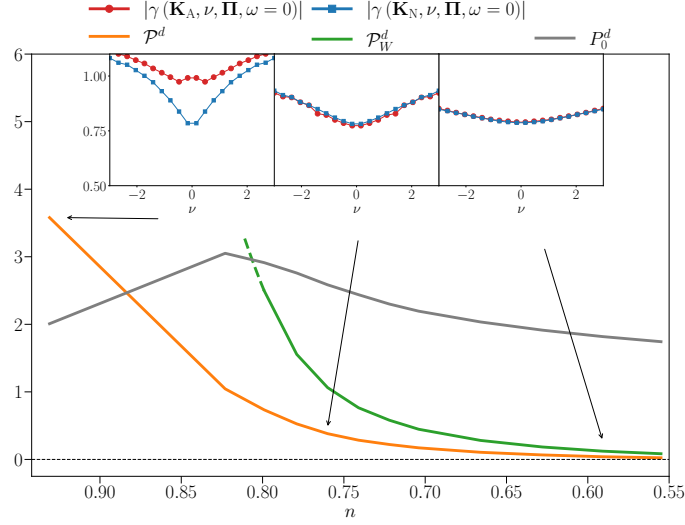

FIG. 7: 16-site DCA calculation with parameters  $t = 1$ ,  $U = 4t$ ,  $t' = 0$ , and  $T = 0.05t$ . Colors as in Fig. 2 of the main text.

As a supplement to the results at strong coupling in the main text and Sec. IIIB, we present a doping scan for weak/intermediate coupling with  $U = 4t$ ,  $t' = 0$ , and  $T = 0.05t$  in Fig. 7. Like in Fig. 2 of the main text, the pairing susceptibilities  $\mathcal{P}^d$ ,  $\mathcal{P}_W^d$  and the spin-fermion vertex  $\gamma$  are shown (insets). In contrast to strong coupling (see Fig. 2 of the main text), as we approach half filling for weak/intermediate coupling,  $|\gamma|$  at the antinodal point increases only moderately, forming only a weak dichotomy where  $|\gamma| \lesssim 1$  for node and antinode alike (left inset). As the result, setting  $|\gamma|$  to 1 enhances the pairing susceptibility also for small doping (green line).

### D. Effective spin-fermion coupling

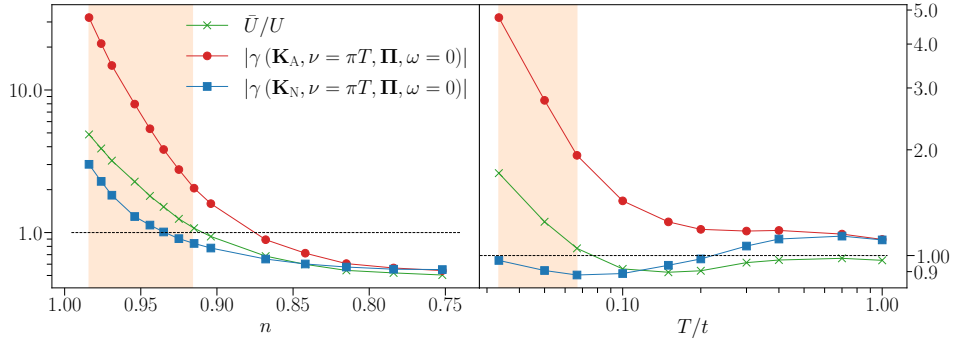

FIG. 8: Effective spin-fermion coupling  $\bar{U}/U$  compared with the exact spin-fermion coupling at the lowest Matsubara frequencies. The simulation parameters are those used in Fig. 2 of the main text.

Previous studies used a frequency- and momentum-independent spin-fermion coupling  $\bar{U}/U$  to analyze spin-fluctuation-mediated pairing. Here, we follow the approach of Refs. [7, 8] and use the definition

$$\bar{U}/U = \sqrt{\frac{\sum_{\mathbf{K}\mathbf{K}'} g_{\mathbf{K}}^d \left[ \sum_{\tilde{\mathbf{K}}=\pm\mathbf{K}'} \sum_{\tilde{\nu}=\pm\pi T} \Gamma(\mathbf{K}, \pi T, \tilde{\mathbf{K}}, \tilde{\nu}) \right] g_{\mathbf{K}'}^d}{\sum_{\mathbf{K}\mathbf{K}'} g_{\mathbf{K}}^d \left[ \sum_{\tilde{\mathbf{K}}=\pm\mathbf{K}'} \sum_{\tilde{\nu}=\pm\pi T} \Gamma^W(\mathbf{K}, \pi T, \tilde{\mathbf{K}}, \tilde{\nu}) \right] g_{\mathbf{K}'}^d}}, \quad (\text{S25})$$

where

$$\Gamma_{KK'}^W = -\frac{3}{2}W_{-K'-K} - \frac{3}{2}W_{K'-K} - 3U, \quad (\text{S26})$$

which is obtained by setting  $\gamma = 1$  in Eq. (S16).

We verified that the  $\bar{U}$  obtained in this way is numerically identical to the  $\bar{U}$  from the particle-particle  $\uparrow\downarrow$  channel, as described in Refs. [7, 8]. As shown in Fig. 8,  $\bar{U}/U$  (green crosses) provides a reasonable approximation for the static ( $\omega = 0$ ) component of  $|\gamma|$  only in the overdoped regime or at high temperatures. As a side note, using this isotropic and frequency-independent spin-fermion coupling in the expression for  $\hat{P}$  in Eq. (S22) only gives meaningful results for overdoping or weak coupling (not shown). A momentum-dependent but frequency-independent estimation of the spin-fermion coupling may be worth testing, but is beyond the scope of this work.

### E. Pair breaking versus attraction

The spin-fermion vertex  $\gamma$  enhances the glue in Eq. (S16), but also pair breaking through the electronic self-energy, which it enters via Hedin's equation [28]. An important question is which effect wins over the other. To probe the impact of  $\gamma$  on superconductivity in the pseudogap regime, we manipulate the static component, namely,  $\gamma_{KQ} \rightarrow (1 + \alpha\delta_\omega)\gamma_{KQ}$ . We include this modification into the pairing glue (S16) as

$$\Gamma_{KK'}^{sf} \rightarrow -\frac{3}{2}(1 + \alpha\delta_{\nu'+\nu})^2|\gamma_{K,-K'-K}|^2W_{-K'-K} - \frac{3}{2}(1 + \alpha\delta_{\nu'-\nu})^2|\gamma_{K,K'-K}|^2W_{K'-K} - 3U. \quad (\text{S27})$$

Notice that we do not renormalize  $W$ , for which we use the original DCA result.

The Fierz ambiguity allows to represent the self-energy in terms of charge, spin, or ( $s$ -wave) particle-particle fluctuations; see also the supplemental material of Ref. [25]. To maximize the pair-breaking effect of  $\gamma$  on the self-energy, we choose the spin picture. The modification of  $\gamma$  then changes  $\Sigma$  as follows,

$$\Sigma(\mathbf{K}, \nu) \rightarrow \Sigma(\mathbf{K}, \nu) - \alpha \frac{1}{\beta N_c} \sum_{\mathbf{Q}} G(\mathbf{K} + \mathbf{Q}, \nu) W(\mathbf{Q}, \omega = 0) \gamma(\mathbf{K}, \mathbf{Q}, \nu, \omega = 0). \quad (\text{S28})$$

Here, we do not take further renormalization of  $G$  and  $W$  on the right-hand-side into account, that is, they (and  $\Sigma, \gamma$  on the right-hand-side) are taken from the DCA calculation.

We use Eq. (S28) for  $\hat{\chi}^0$  in the ladder equation (S18) to calculate  $\hat{\chi}^r$  for a given  $\alpha$  (notice that  $\hat{\Gamma}^r$  is also not renormalized and taken from the DCA calculation). We then calculate the pairing susceptibility by inserting (S27) into Eq. (S22). The gray line in Fig. 9 shows that the bare pairing susceptibility  $\mathcal{P}_{0,\alpha}^d$  is slightly suppressed for  $\alpha > 0$  due to stronger pair breaking, as expected. However, the dressed susceptibility  $\mathcal{P}_\alpha^d$  (green) quickly diverges when  $\alpha$  increases, highlighting that pair breaking is overcompensated by attraction. For  $\alpha < 0$ , superconductivity is suppressed.

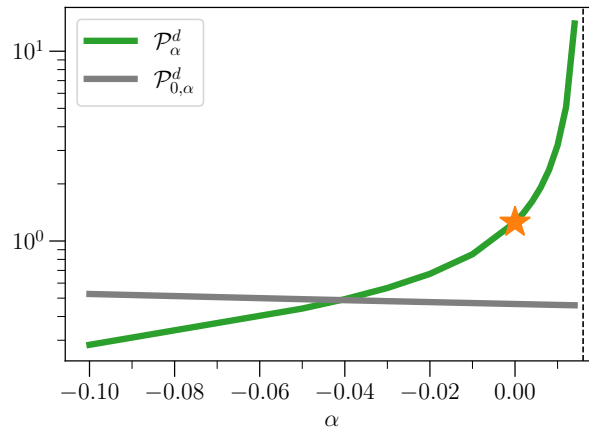

FIG. 9: The  $d$ -wave pairing susceptibility  $\mathcal{P}_\alpha^d$  (green) and the bare susceptibility  $\mathcal{P}_{0,\alpha}^d$  (gray) in the pseudogap regime as a function of  $\alpha$ , which slightly modifies the static spin-fermion vertex via  $\gamma_{KQ} \rightarrow (1 + \alpha\delta_\omega)\gamma_{KQ}$ . The orange star at  $\alpha = 0$  represents the DCA calculation  $\delta = 0.075$  and  $T = 0.05t$ , corresponding to the orange stars in the main text. At  $\alpha = 0.016$  (black dashed line), a divergence of  $\mathcal{P}_\alpha^d$  is observed.

## F. Comments on previous studies

To our best knowledge, previous studies did not observe the enhanced antinodal spin-fermion coupling as presented here. Refs. [29, 30] may not have reached low enough temperatures or sufficiently strong correlation regimes. Further, the methods employed in Refs. [31, 32] may possibly not capture this effect, because they use metallic DMFT calculations as a starting point, and where  $\gamma$  is suppressed [33]. Such a suppression would limit them to the weak correlation regime of superconductivity which applies in DCA only for overdoping. Instead, for underdoping DCA predicts a novel regime of strongly correlated superconductivity marked by  $|\gamma|^2 \gg 1$  for antinodal fermions, see the main text. On the other hand, DCA may overestimate the importance of Kondo physics. It seems therefore appealing to evaluate  $\gamma$  within numerically exact approaches to the Hubbard model [34].

## IV. ADDITIONAL DETAILS ON DCA CALCULATIONS

In this section, we provide additional details on the DCA calculations performed in this study. Fig. 10 presents the momentum tiling of the DCA clusters used. Fig. 11 offers further supporting data to illustrate the opening of the pseudogap at  $n = 0.925$ , which corresponds to the density used in the temperature scan discussed in the main text. In the main text, the condition  $-\text{Im}\Sigma(\mathbf{K}_A, \pi T) > -\text{Im}\Sigma(\mathbf{K}_A, 3\pi T)$  is used to identify insulating behavior at the antinode, while  $-\text{Im}\Sigma(\mathbf{K}_N, \pi T) < -\text{Im}\Sigma(\mathbf{K}_N, 3\pi T)$  is used to identify metallic behavior at the node. Together, these conditions signal the opening of the pseudogap. In Fig. 11, we show the negative of the self-energy,  $-\text{Im}\Sigma(\mathbf{K}, \nu_j)$ , at the antinode (top panel) and node (bottom panel) as a function of the Matsubara frequency index  $j$ , where  $\nu_j = (2j + 1)\pi T$ . It is clear that the pseudogap condition mentioned above is satisfied for temperatures below  $T = 0.067t$ . This figure confirms the pseudogap opening for the primary data presented in the main text, which corresponds to  $T = 0.05t$ .

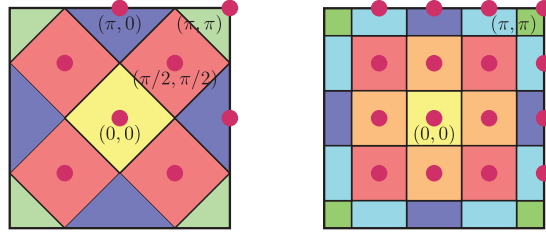

FIG. 10: Momentum tiling of the DCA clusters: 8-site cluster (left) and 16-site cluster (right). Adapted from Ref. [35].

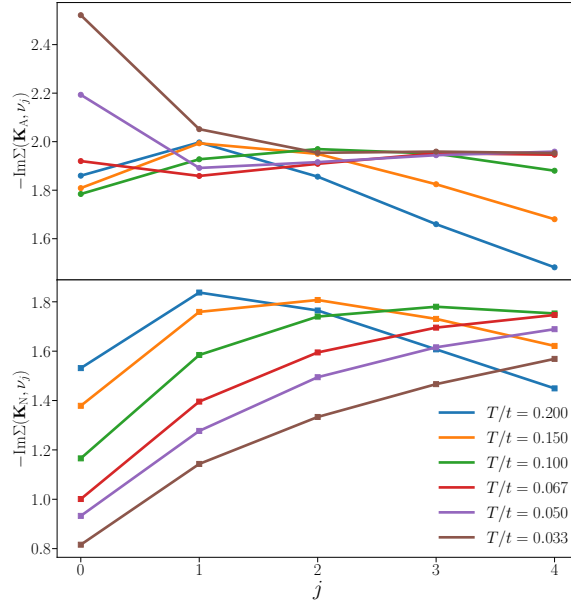

FIG. 11: Self-energy at the antinode (top) and node (bottom) for various temperatures at filling  $\delta = 0.075$ . The simulation parameters are those used in Fig. 2 of the main text.

- 
- [1] D.J. Scalapino, “The case for  $d_{x^2-y^2}$  pairing in the cuprate superconductors,” *Physics Reports* **250**, 329–365 (1995).
  - [2] Friedrich Krien, Angelo Valli, and Massimo Capone, “Single-boson exchange decomposition of the vertex function,” *Phys. Rev. B* **100**, 155149 (2019).
  - [3] Xi Chen, J. P. F. LeBlanc, and Emanuel Gull, “Superconducting fluctuations in the normal state of the two-dimensional hubbard model,” *Phys. Rev. Lett.* **115**, 116402 (2015).
  - [4] Thomas A. Maier, Mark Jarrell, Thomas Pruschke, and Matthias Hettler, “Quantum cluster theories,” *Rev. Mod. Phys.* **77**, 1027–1080 (2005).
  - [5] T. A. Maier, M. S. Jarrell, and D. J. Scalapino, “Structure of the pairing interaction in the two-dimensional hubbard model,” *Phys. Rev. Lett.* **96**, 047005 (2006).
  - [6] Thomas A. Maier, M. Jarrell, and D. J. Scalapino, “Pairing interaction in the two-dimensional hubbard model studied with a dynamic cluster quantum monte carlo approximation,” *Phys. Rev. B* **74**, 094513 (2006).
  - [7] T. A. Maier, A. Macridin, M. Jarrell, and D. J. Scalapino, “Systematic analysis of a spin-susceptibility representation of the pairing interaction in the two-dimensional hubbard model,” *Phys. Rev. B* **76**, 144516 (2007).
  - [8] T. A. Maier, M. Jarrell, and D. J. Scalapino, “Spin susceptibility representation of the pairing interaction for the two-dimensional hubbard model,” *Phys. Rev. B* **75**, 134519 (2007).
  - [9] M. H. Hettler, A. N. Tahvildar-Zadeh, M. Jarrell, T. Pruschke, and H. R. Krishnamurthy, “Nonlocal dynamical correlations of strongly interacting electron systems,” *Phys. Rev. B* **58**, R7475–R7479 (1998).
  - [10] M. H. Hettler, M. Mukherjee, M. Jarrell, and H. R. Krishnamurthy, “Dynamical cluster approximation: Nonlocal dynamics of correlated electron systems,” *Phys. Rev. B* **61**, 12739–12756 (2000).
  - [11] A. N. Rubtsov, V. V. Savkin, and A. I. Lichtenstein, “Continuous-time quantum monte carlo method for fermions,” *Phys. Rev. B* **72**, 035122 (2005).
  - [12] Philipp Werner, Armin Comanac, Luca de’ Medici, Matthias Troyer, and Andrew J. Millis, “Continuous-time solver for quantum impurity models,” *Phys. Rev. Lett.* **97**, 076405 (2006).
  - [13] E. Gull, P. Werner, O. Parcollet, and M. Troyer, “Continuous-time auxiliary-field monte carlo for quantum impurity models,” *Europhysics Letters* **82**, 57003 (2008).
  - [14] Emanuel Gull, Andrew J. Millis, Alexander I. Lichtenstein, Alexey N. Rubtsov, Matthias Troyer, and Philipp Werner, “Continuous-time monte carlo methods for quantum impurity models,” *Rev. Mod. Phys.* **83**, 349–404 (2011).
  - [15] Emanuel Gull, Peter Staar, Sebastian Fuchs, Phani Nukala, Michael S. Summers, Thomas Pruschke, Thomas C. Schulthess, and Thomas Maier, “Submatrix updates for the continuous-time auxiliary-field algorithm,” *Phys. Rev. B* **83**, 075122 (2011).
  - [16] D. J. Scalapino, “A common thread: The pairing interaction for unconventional superconductors,” *Rev. Mod. Phys.* **84**, 1383–1417 (2012).
  - [17] Motoharu Kitatani, Ryotaro Arita, Thomas Schäfer, and Karsten Held, “Strongly correlated superconductivity with long-range spatial fluctuations,” *Journal of Physics: Materials* **5**, 034005 (2022).
  - [18] T. Schäfer, G. Rohringer, O. Gunnarsson, S. Ciuchi, G. Sangiovanni, and A. Toschi, “Divergent precursors of the mott-hubbard transition at the two-particle level,” *Phys. Rev. Lett.* **110**, 246405 (2013).
  - [19] O. Gunnarsson, T. Schäfer, J. P. F. LeBlanc, J. Merino, G. Sangiovanni, G. Rohringer, and A. Toschi, “Parquet decomposition calculations of the electronic self-energy,” *Phys. Rev. B* **93**, 245102 (2016).
  - [20] T. Schäfer, S. Ciuchi, M. Wallerberger, P. Thunström, O. Gunnarsson, G. Sangiovanni, G. Rohringer, and A. Toschi, “Nonperturbative landscape of the mott-hubbard transition: Multiple divergence lines around the critical endpoint,” *Phys. Rev. B* **94**, 235108 (2016).
  - [21] J. Vučković, N. Wentzell, M. Ferrero, and O. Parcollet, “Practical consequences of the luttinger-ward functional multi-valuedness for cluster DMFT methods,” *Phys. Rev. B* **97**, 125141 (2018).
  - [22] For matrix-valued equations like the BSE, the presence of eigenvalues exactly equal to 1 does still not necessarily guarantee a divergent response function. This is because, for example, an exact antisymmetry of the corresponding eigenvectors can cancel out the divergence, as explained in Ref. [36].
  - [23] Friedrich Krien, Anna Kauch, and Karsten Held, “Tiling with triangles: parquet and  $GW\gamma$  methods unified,” *Phys. Rev. Research* **3**, 013149 (2021).
  - [24] Notice that  $\chi_Q^{\text{sp}}$  is defined as a negative quantity (see Eq. (S5b) in Ref.[25]).
  - [25] Yang Yu, Sergei Isakov, Emanuel Gull, Karsten Held, and Friedrich Krien, “Unambiguous fluctuation decomposition of the self-energy: Pseudogap physics beyond spin fluctuations,” *Phys. Rev. Lett.* **132**, 216501 (2024).
  - [26] Friedrich Krien and Anna Kauch, “The plain and simple parquet approximation: single-and multi-boson exchange in the two-dimensional hubbard model,” *The European Physical Journal B* **95** (2022), 10.1140/epjb/s10051-022-00329-6.
  - [27] Friedrich Krien and Angelo Valli, “Parquetlike equations for the hedin three-leg vertex,” *Phys. Rev. B* **100**, 245147 (2019).
  - [28] Lars Hedin, “New method for calculating the one-particle green’s function with application to the electron-gas problem,” *Phys. Rev.* **139**, A796–A823 (1965).
  - [29] Z. B. Huang, W. Hanke, and E. Arrighi, “Role of vertex corrections in the spin-fluctuation-mediated pairing mechanism,” *Europhysics Letters (EPL)* **71**, 959–965 (2005).
  - [30] Z. B. Huang, W. Hanke, E. Arrighi, and A. V. Chubukov, “Renormalization of the electron-spin-fluctuation interaction in the  $t-t'-u$  hubbard model,” *Phys. Rev. B* **74**, 184508 (2006).
  - [31] Motoharu Kitatani, Thomas Schäfer, Hideo Aoki, and Karsten Held, “Why the critical temperature of high- $T_c$  cuprate superconductors is so low: The importance of the dynamical vertex structure,” *Phys. Rev. B* **99**, 041115(R) (2019).

- [32] Friedrich Krien, Paul Worm, Patrick Chalupa-Gantner, Alessandro Toschi, and Karsten Held, “Explaining the pseudogap through damping and antidamping on the fermi surface by imaginary spin scattering,” *Communications Physics* **5**, 336 (2022).
- [33] Viktor Harkov, Alexander I. Lichtenstein, and Friedrich Krien, “Parametrizations of local vertex corrections from weak to strong coupling: Importance of the hedin three-leg vertex,” *Phys. Rev. B* **104**, 125141 (2021).
- [34] Fedor Simkovic IV, Riccardo Rossi, and Michel Ferrero, “Two-dimensional hubbard model at finite temperature: Weak, strong, and long correlation regimes,” *Phys. Rev. Res.* **4**, 043201 (2022).
- [35] E. Gull, M. Ferrero, O. Parcollet, A. Georges, and A. J. Millis, “Momentum-space anisotropy and pseudogaps: A comparative cluster dynamical mean-field analysis of the doping-driven metal-insulator transition in the two-dimensional hubbard model,” *Phys. Rev. B* **82**, 155101 (2010).
- [36] Erik G. C. P. van Loon, Friedrich Krien, and Andrey A. Katanin, “Bethe-salpeter equation at the critical end point of the mott transition,” *Phys. Rev. Lett.* **125**, 136402 (2020).
